# Supplementary material for: Orthogonal Causal Calibration
Source: arXiv:2406.01933 source file (2025-04-30)
Supplement: Supplementary file 1 [file worked_eg.tex]

\begin{example}[Example~\ref{..} (contd.)]
 This loss is clearly not orthogonal with respect to $\mu$. However, it admits a well-known translation into an orthogonalized loss which uses an extra nuisance function: the propensity score $\pi(x) = \P(A = 1|X = x)$. This orthogonalized loss is given by
\begin{align*}
    \wt{\ell}_{sq}(\theta, (\mu, \pi); z) = \frac{1}{2}\left(\theta(x) - \mu(1, x) + \mu(0, x) - \left(\frac{a}{\pi(x)} - \frac{1 - a}{1 - \pi(x)}\right)(y - \mu(a, x))\right)^2
\end{align*}
which is often known as the doubly-robust loss.\cj{TODO: let's actually derive this by talking about what $g_0$ and $b(w)$ looks like for this setting. Hmm it seems like we kind of do this below. I think this part can use more passes. Happy to go through this part after chatting a bit later} Intuitively, we can think of this as measuring the squared error between $\theta(x)$ and a ``pseudo-outcome" given by 
\begin{align*}
   \chi((\mu, \pi); z) =  \mu(1, x) + \mu(0, x) - \left(\frac{a}{\pi(x)} - \frac{1 - a}{1 - \pi(x)}\right)(y - \mu(a, x)).
\end{align*}
The pseudo-outcome is equal in expectation to $CATE(x)$ as long as either $\mu$ or $\pi$ is perfectly estimated ($\mu = \mu_0$ or $\pi = \pi_0$).
The most important example of a loss that can be made universally orthogonal is the square loss $\ell_{sq}(\theta, \mu; z) := \frac{1}{2}(\theta(x) - \mu(1, x) + \mu(0, x))^2$, where we have $\mu(a, x) := \E[Y(a) \mid X = x] = \E[Y \mid X = x, A = a]$ as our nuisance. Quite clearly, $\ell_{sq}$ has as its minimizer $\theta_0$ the conditional average treatment effect. The orthogonalized version of $\ell_{sq},$ denoted by $\wt{\ell}_{sq}$, is given by
\[
\wt{\ell}_{sq}(\theta, (\mu, \pi); z) = \ell_{sq}(\theta, \mu; z) - \theta(x)\cdot\left(\left(\frac{a}{\pi(x)} - \frac{1 - a}{1 - \pi(x)}\right)(y - \mu(a, x))\right),
\]
where we have enforced the identity $b = \frac{a}{\pi(x)} - \frac{1 - a}{1 - \pi(x)}$ for some function $\pi : \calX \rightarrow [0, 1]$. The true, unknown additional nuisance $b_0$ in this setting is in fact given by $b_0(a, x) = \frac{a}{\pi_0(x)} - \frac{1 - a}{1 - \pi_0(x)}$, where $\pi_0(x) := \P(A = 1 \mid X = x) \in [0, 1]$ is the unknown propensity score. We note that $\wt{\ell}_{sq}$ is ``equivalent'' in a certain sense to the commonly-used doubly robust loss, a fact that will be discussed in Section~\ref{sec:alg} below. A straightforward computation shows that
\[
\E[\partial \wt{\ell}_{sq}(\theta, (\mu, \pi); Z) \mid X] =  \theta(X) - g(1, X) + g(0, X) - \E\left[\left(\frac{A}{\pi(X)} - \frac{(1 - A)}{1 - \pi(X)}\right)(Y  - \mu(A, X))\mid X\right], 
\]
and so subsequently taking the Gateaux derivative with respect to $\wt{g} = (\mu, b)$ yields a quantity that is independent of the chosen estimator $\theta : \calX \rightarrow \R$. Thus, the orthogonalized square loss actually satisfies universal orthogonality.\cj{I think the last part seems a bit rushed. Just for my own sake, trying to write down the structure that we may want.
\begin{enumerate}
    \item show that $\ell_{sq}$ by itself is not universally orthogonal.
    \item show how to derive the orthogonalized loss $\wt{\ell}_{sq}$. 
    \item show that the new orthogonalized loss is actually universally orthogonal
    \item mention that this is actually equivalent to doubly robust loss, which we'll discuss in Section 6.
\end{enumerate}}
\end{example}

\begin{example}[Example~\ref{...} (contd.)]
The orthogonalized loss can be written as
\[
\wt{\ell}_{cd}(\theta, (\mu, \pi); z) = \frac{1}{2}(\theta(x) - \partial_a \mu(a, x))^2 - \theta(x)\cdot\left(\frac{\partial_a \pi(a \mid x)}{\pi(a \mid x)}(\mu(a, x) - y)\right),
\]
where we have enforced that estimates $b(a, x) := \frac{\partial_a \pi(a \mid x)}{\pi(a \mid x)}$ for some Lebesgue density $\pi(a \mid x)$. It is clear that
\begin{align*}
\E[\partial \wt{\ell}(\theta, \wt{g}; Z) \mid X] &= \E[\theta(X) - \partial_a \mu(A, X)\mid X] - \E\left[\frac{\partial_a \pi(A \mid X)}{\pi(A \mid X)}(\mu(A, X) - Y) \mid X\right],
\end{align*}
so by the same reasoning as above, the Gateaux derivative at any point along any direction is independent of the estimator $\theta(x)$. 

Thus, to show universal orthogonality, it suffices to exhibit a value for the true, unknown nuisance $b_0$. In this setting, $b_0(a, x) = \frac{\partial_a \pi_0(a \mid x)}{\pi_0(a \mid x)}$, where $\pi_0(a \mid x)$ is the Lebesgue density of $A$ given $X = x$, i.e.\ $\pi_0(a \mid x)$ is defined almost everywhere by $\int_a^b\pi_0(a \mid x)da = \P(A \in [a, b] \mid X = x)$. This should be viewed as a continuous analogue of the propensity score leveraged in the case of square loss. Indeed, a simple computation shows that
\begin{align*}
&\E\left[\frac{\partial_a \pi_0(A \mid X)}{\pi_0(A \mid X)}(\mu(A, X) - Y) \mid X\right]\\
&\qquad = \int_0^1 \frac{\partial_a \pi_0(a \mid X)}{\pi_0(a \mid X)}(\mu(a, X) - \mu_0(a, X))\pi_0(a \mid X) da \\
&\qquad = \int_0^1 \partial_a \pi_0(a \mid X)(\mu(a, X) - \mu_0(a, X))da \\
&\qquad = \left[\pi_0(a \mid X)(\mu(a, X) - \mu_0(a, X))\right]_{a = 0}^1 - \int_0^1(\partial_a\mu(a, X) - \partial_a\mu_0(a, X))\pi_0(a \mid X)da \\
&\qquad = E\left[\partial_a(\mu_0(A, X) - \mu(A, X))\mid X\right],
\end{align*}
where in the above we apply integration by parts and implicitly assume the boundary conditions $\pi(0 \mid x) = \pi(1 \mid x) = 0$ for all $x \in \calX$. With this, it isn't hard to see that
\begin{align*}
&D_{\mu}\E[\partial \wt{\ell}(\theta, (\mu_0, b_0); Z) \mid X](\mu - \mu_0) \\
&\qquad =  - \E[\partial_a (\mu(A, X) - \mu_0(A, X))\mid X] - \E\left[\frac{\partial_a \pi_0(A \mid X)}{\pi_0(A \mid X)}(\mu(A, X) - Y) \mid X\right] \\
&\qquad = - \E\left[\partial_a (\mu(A, X) - \mu_0(A, x) \mid X\right] - \E\left[\partial_a(\mu_0(A, X) - \mu(A, X))\mid X\right] \\
&\qquad = 0.
\end{align*}
Another straightforward computation yields that $D_{b}\E[\partial \wt{\ell}(\theta, \wt{g}_0; Z) \mid X](b - b_0)$ vanishes as well. Thus, we have argued that the loss is universally orthogonal.
\end{example}

\begin{example}[Example~\ref{..} (contd.)]
In straightforward manner, one can verify that, when we enforce estimates of the form $g = \frac{p}{q}$, we have 
\begin{align*}
D_{g}\E[\partial \ell_{le}(\theta, g_0; Z) \mid X](g - g_0) &= \left(\frac{p}{q} - \frac{p_0}{q_0}\right)(X) \\
&= \frac{p(X)q_0(X)}{q(X)q_0(X)} - \frac{p_0(X)q(X)}{q(X)q_0(X)} \\
&= \frac{1}{q_0(X)}\left(\frac{p(X)q_0(X)}{q(X)} - \frac{p_0(X)q(X)}{q(X)}\right) \\
&= \E\left[\frac{1}{q_0(X)}\left(\frac{p(X)D(A - \pi_0(X))}{q(X)} - Y(A- \pi_0(X))\right) \mid X = x\right],
\end{align*}
and thus the orthogonalized loss can be written as
\[
\wt{\ell}_{le}(\theta, (p, q); z) = \ell_{le}(\theta, (p, q); z) - \frac{1}{q(x)}\left(\frac{p(x) d (a - \pi_0(x))}{q(x)} - y(a - \pi_0(x))\right),
\]
where we note the additional nuisance (i.e.\ Riesz representer) that must be learned is none other than $b_0(x) = q_0(x)$. Using the notion of ``equivalent loss'' and Lemma~\ref{lem:equiv_loss}, we see that $\wt{\ell}_{le}$ actually shares the same minimizer and orthogonality properties as the squared loss $\wt{\ell}_{le}^{eq}(\theta, (p, q); z)$ given by
\[
\wt{\ell}_{le}^{eq}(\theta, (p, q); z) = \frac{1}{2}(\theta(x) - \chi((p, q); z))^2,
\]
where in this setting pseudo-outcomes are given as
\[
\chi((p, q); z) := \frac{p(x)}{q(x)} + \frac{1}{q(x)^2}(a - \pi_0(x))\left(d\cdot p(x) - y\right),
\]
which is precisely as is seen in \citet{lan2023causal}.
\end{example}
